# Supplementary material for: Mitigating Frequency Bias in Next-Basket Recommendation via Deconfounders
Source: arXiv:2211.09072 source file (2022-11-16)
Supplement: Supplementary file 1 [file 6-Appendices.tex]

\section{Appendix}

\subsection{Pilot Study}
In this section we show the performance of pilot study to show the existence of frequency bias in the dataset. 

\subsection{Explaining Biases in the Dataset}
In this section we will detailedly explain why confounders render biases and noises in recommendations.

Confounders are variables that affect both the cause and effect simultaneously. They are widely studied since they can render biased results and even wrong conclusions in statistics. Even in prediction tasks, they can introduce biases and noises into the datasets.

the biases in the dataset, including why there would be biases, how does a bias looks like and what would happen if we do nothing to the bias.

According to \cite{wang2019blessings,holland1986statistics}

\subsection{Select Proper PIF}
In this section we introduce methods to calculate PIF along the historical purchasing records.

\subsection{More Experiments}
